# Supplementary material for: Learning From An Optimization Viewpoint
Source: arXiv:1204.4145 source file (2012-04-18)
Supplement: Supplementary file 1 [file appendix.tex]

\chapter[\Large Banach Space Geometry]{
Banach Space Geometry}\label{app:banach}
